# Supplementary material for: Rumor Spreading with Bounded In-Degree
Source: arXiv:1506.00828 source file (2015-09-22)
Supplement: Supplementary file 1 [file appendix-proofs.tex]

%%% Local Variables: 
%%% mode: latex
%%% TeX-master: "rumorSpreading_lipics"
%%% End: 

%%% Local Variables: 
%%% mode: latex
%%% TeX-master: "rumorSpreading_lipics"
%%% End: 
